# Supplementary material for: DORA Explorer: Improving the Exploration Ability of LLMs Without Training
Source: arXiv:2604.17244 source file (2026-08-11)
Supplement: Supplementary file 1 [file Appendix_mab_full_table.tex]

\begin{table*}[h!]
\centering
\setlength{\tabcolsep}{3.5pt}
\renewcommand{\arraystretch}{1.5}
\begin{adjustbox}{max width=\textwidth}
\begin{tabular}{l*{13}{c}}
\toprule
\multirow{2}{*}{\diagbox[width=8em, height=3em]{\textbf{Metric}}{\textbf{Method}}} 
& \multicolumn{4}{c}{Classic Strategies} 
& \multicolumn{6}{c}{Temperature ($\tau$)} 
& \multicolumn{3}{c}{Learned Policies} \\
\cmidrule(lr){2-5} \cmidrule(lr){6-11} \cmidrule(lr){12-14}

& UCB
& TS
& Greedy
& $\varepsilon$-Greedy
& $\tau=0$
& $\tau=0.3$
& $\tau=0.7$
& $\tau=1$
& $\tau=1.5$
& $\tau=2$
& $\tau$-Policy
& DORA ($\lambda$)
& DORA (auto) \\
\midrule

Mean Avg Reward
& \cellcolor{greenDark}\textcolor{white}{0.531}
& \cellcolor{greenMed}0.512
& \cellcolor{greenLight}0.506
& \cellcolor{greenLight!70}0.490
& \cellcolor{greenPale}0.410
& \cellcolor{greenPale}0.410
& \cellcolor{greenPale}0.410
& \cellcolor{greenPale!80}0.401
& \cellcolor{greenLight!60}0.440
& \cellcolor{greenPale!60}0.393
& \cellcolor{greenLight!50}0.433
& \cellcolor{greenMed}\textbf{\textcolor{white}{0.514}}
& \cellcolor{greenLight}0.462 \\

SuffFailFreq($T$/2)
& \cellcolor{greenMed}0.02
& \cellcolor{greenDark}\textcolor{white}{0.00}
& \cellcolor{greenLight!70}0.42
& \cellcolor{greenLight}0.30
& \cellcolor{greenPale}0.90
& \cellcolor{greenPale}0.90
& \cellcolor{greenPale}0.90
& \cellcolor{greenPale!80}0.95
& \cellcolor{greenLight}0.25
& \cellcolor{greenDark}\textcolor{white}{0.00}
& \cellcolor{greenLight!60}0.10
& \cellcolor{greenDark}\textcolor{white}{0.00}
& \cellcolor{greenLight!70}0.60 \\

Best arm Frac
& \cellcolor{greenDark}\textcolor{white}{0.66}
& \cellcolor{greenMed}0.57
& \cellcolor{greenLight}0.53
& \cellcolor{greenLight!70}0.455
& \cellcolor{greenPale}0.10
& \cellcolor{greenPale}0.10
& \cellcolor{greenPale}0.10
& \cellcolor{greenPale!80}0.04
& \cellcolor{greenLight}0.301
& \cellcolor{greenLight!60}0.442
& \cellcolor{greenLight!50}0.434
& \cellcolor{greenMed}0.585
& \cellcolor{greenLight!70}0.356 \\

Cum Regret
& \cellcolor{greenDark}\textcolor{white}{13.68}
& \cellcolor{greenMed}17.16
& \cellcolor{greenLight}18.90
& \cellcolor{greenLight!70}21.80
& \cellcolor{greenPale}36.00
& \cellcolor{greenPale}36.00
& \cellcolor{greenPale}36.00
& \cellcolor{greenPale!80}38.39
& \cellcolor{greenLight}28.45
& \cellcolor{greenLight!60}25.70
& \cellcolor{greenLight!50}24.41
& \cellcolor{greenMed}16.61
& \cellcolor{greenLight!60}25.77 \\

Invalid Commands
& \cellcolor{greenDark}\textcolor{white}{0}
& \cellcolor{greenDark}\textcolor{white}{0}
& \cellcolor{greenDark}\textcolor{white}{0}
& \cellcolor{greenDark}\textcolor{white}{0}
& \cellcolor{greenDark}\textcolor{white}{0}
& \cellcolor{greenDark}\textcolor{white}{0}
& \cellcolor{greenDark}\textcolor{white}{0}
& \cellcolor{greenDark}\textcolor{white}{0}
& \cellcolor{greenLight}6.15
& \cellcolor{greenPale!80}38.35
& \cellcolor{greenLight!70}21.2
& \cellcolor{greenDark}\textcolor{white}{0}
& \cellcolor{greenDark}\textcolor{white}{0} \\

\bottomrule
\end{tabular}
\end{adjustbox}
\caption{Performance comparison across classical bandit strategies, temperature-based sampling, and learned exploration policies. Results are averaged over multiple runs (1000 for classical methods, 20 for others). Darker green indicates better performance. Model: \texttt{Meta Llama 3.1 8B}.}
\end{table*}



% \begin{table}[h!]
% \centering
% \setlength{\tabcolsep}{3.5pt}
% \renewcommand{\arraystretch}{1.5}
% \begin{adjustbox}{max width=\textwidth}
% \begin{tabular}{l*{13}{c}}
% \toprule
% \multirow{2}{*}{\diagbox[width=8em, height=3em]{\textbf{Metric}}{\textbf{Method}}} 
% & \multicolumn{4}{c}{Classic Strategies} 
% & \multicolumn{6}{c}{Temperature ($\tau$)} 
% & \multicolumn{3}{c}{Learned Policies} \\
% \cmidrule(lr){2-5} \cmidrule(lr){6-11} \cmidrule(lr){12-14}

% & UCB
% & TS
% & Greedy
% & $\varepsilon$-Greedy
% & $\tau=0$
% & $\tau=0.3$
% & $\tau=0.7$
% & $\tau=1$
% & $\tau=1.5$
% & $\tau=2$
% & $\tau$ Policy
% & DORA ($\lambda$-sched)
% & DORA (auto) \\
% \midrule

% Mean Avg Reward
% & \cellcolor[HTML]{27AE60}\textcolor{white}{0.531}
% & \cellcolor[HTML]{82CA60}0.512
% & \cellcolor[HTML]{A8D96A}0.506
% & \cellcolor[HTML]{F1C40F}0.490
% & \cellcolor[HTML]{E74C3C}\textcolor{white}{0.410}
% & \cellcolor[HTML]{E74C3C}\textcolor{white}{0.410}
% & \cellcolor[HTML]{E74C3C}\textcolor{white}{0.410}
% & \cellcolor[HTML]{C0392B}\textcolor{white}{0.401}
% & \cellcolor[HTML]{D4AC0D}0.440
% & \cellcolor[HTML]{E67E22}0.393
% & \cellcolor[HTML]{F1C40F}0.433
% & \cellcolor[HTML]{6CBF60}\textbf{0.514}
% & \cellcolor[HTML]{2ECC71}\textcolor{white}{0.462} \\

% SuffFailFreq($T$/2)
% & \cellcolor[HTML]{82CA60}0.02
% & \cellcolor[HTML]{27AE60}\textcolor{white}{0.00}
% & \cellcolor[HTML]{F1C40F}0.42
% & \cellcolor[HTML]{D4AC0D}0.30
% & \cellcolor[HTML]{E74C3C}\textcolor{white}{0.90}
% & \cellcolor[HTML]{E74C3C}\textcolor{white}{0.90}
% & \cellcolor[HTML]{E74C3C}\textcolor{white}{0.90}
% & \cellcolor[HTML]{C0392B}\textcolor{white}{0.95}
% & \cellcolor[HTML]{F1C40F}0.25
% & \cellcolor[HTML]{27AE60}\textcolor{white}{0.00}
% & \cellcolor[HTML]{6CBF60}\textcolor{white}{0.10}
% & \cellcolor[HTML]{27AE60}\textcolor{white}{0.00}
% & \cellcolor[HTML]{E67E22}0.60 \\

% Best arm Frac
% & \cellcolor[HTML]{27AE60}\textcolor{white}{0.66}
% & \cellcolor[HTML]{82CA60}0.57
% & \cellcolor[HTML]{A8D96A}0.53
% & \cellcolor[HTML]{F1C40F}0.455
% & \cellcolor[HTML]{E74C3C}\textcolor{white}{0.10}
% & \cellcolor[HTML]{E74C3C}\textcolor{white}{0.10}
% & \cellcolor[HTML]{E74C3C}\textcolor{white}{0.10}
% & \cellcolor[HTML]{C0392B}\textcolor{white}{0.04}
% & \cellcolor[HTML]{D4AC0D}0.301
% & \cellcolor[HTML]{A8D96A}0.442
% & \cellcolor[HTML]{F1C40F}0.434
% & \cellcolor[HTML]{6CBF60}0.585
% & \cellcolor[HTML]{F39C12}0.356 \\

% Cum Regret
% & \cellcolor[HTML]{27AE60}\textcolor{white}{13.68}
% & \cellcolor[HTML]{82CA60}17.16
% & \cellcolor[HTML]{A8D96A}18.90
% & \cellcolor[HTML]{F1C40F}21.80
% & \cellcolor[HTML]{E74C3C}\textcolor{white}{36.00}
% & \cellcolor[HTML]{E74C3C}\textcolor{white}{36.00}
% & \cellcolor[HTML]{E74C3C}\textcolor{white}{36.00}
% & \cellcolor[HTML]{C0392B}\textcolor{white}{38.39}
% & \cellcolor[HTML]{D4AC0D}28.45
% & \cellcolor[HTML]{F39C12}25.70
% & \cellcolor[HTML]{F1C40F}24.41
% & \cellcolor[HTML]{6CBF60}16.61
% & \cellcolor[HTML]{F39C12}25.77 \\

% Invalid Commands
% & \cellcolor[HTML]{27AE60}0
% & \cellcolor[HTML]{27AE60}0
% & \cellcolor[HTML]{27AE60}0
% & \cellcolor[HTML]{27AE60}0
% & \cellcolor[HTML]{27AE60}0
% & \cellcolor[HTML]{27AE60}0
% & \cellcolor[HTML]{27AE60}0
% & \cellcolor[HTML]{27AE60}0
% & \cellcolor[HTML]{F1C40F}6.15
% & \cellcolor[HTML]{E74C3C}\textcolor{white}{38.35}
% & \cellcolor[HTML]{E67E22}21.2
% & \cellcolor[HTML]{27AE60}0
% & \cellcolor[HTML]{27AE60}0 \\

% \bottomrule
% \end{tabular}
% \end{adjustbox}
% \caption{Performance comparison across classical bandit strategies, temperature-based sampling, and learned exploration policies. Results are averaged over multiple runs (1000 for classical methods, 20 for others). Green indicates better performance, red indicates worse. Model used meta llama}
% \end{table}
