# Supplementary material for: DORA Explorer: Improving the Exploration Ability of LLMs Without Training
Source: arXiv:2604.17244 source file (2026-08-11)
Supplement: Supplementary file 2 [file Appendix_tales_loop_recovery.tex]

\begin{table}[t]
\centering
\setlength{\tabcolsep}{5pt}
\renewcommand{\arraystretch}{1.2}
\begin{tabular}{lcccc}
\toprule
\textbf{Method} & \textbf{Loops Enc.} & \textbf{Loops Rec.} & \textbf{Recovery (\%)} & \textbf{Explore@Loop} \\
\midrule
\multicolumn{5}{c}{\textit{TextWorld}} \\
Zero-shot & 612 & 3 & 0.5 & 0 \\
Prompt Explore & 663 & 5 & 0.8 & 0 \\
CoT & 673 & 24 & 3.6 & 0 \\
ToT & 783 & 8 & 1.0 & 0 \\
DORA (Auto) & 185 & 36 & 19.5 & 36 \\

\midrule
\multicolumn{5}{c}{\textit{ScienceWorld}} \\
Zero-shot & 2551 & 9 & 0.35 & 0 \\
Prompt Explore & 2321 & 10 & 0.43 & 0 \\
CoT & 2621 & 6 & 0.23 & 0 \\
ToT & 2801 & 2 & 0.07 & 0 \\
DORA (Auto) & 1234 & 45 & 3.6 & 11 \\

\midrule
\multicolumn{5}{c}{\textit{AlfWorld}} \\
Zero-shot & 811 & 0 & 0.0 & 0 \\
Prompt Explore & 721 & 1 & 0.1 & 0 \\
CoT & 846 & 1 & 0.1 & 0 \\
ToT & 857 & 0 & 0.0 & 0 \\
DORA (Auto) & 111 & 12 & 10.8 & 27 \\
\bottomrule
\end{tabular}
\caption{Detailed loop statistics, including exploration usage at loop states.}
\label{tab:loop_recovery_full}
\end{table}
